# Supplementary material for: AI Research is not Magic, it has to be Reproducible and Responsible: Challenges in the AI field from the Perspective of its PhD Students
Source: arXiv:2408.06847 source file (2024-08-13)
Supplement: Supplementary file 1 [file Appendix_A_Questions_for_respondents_during_focus_groups_interviews-1.pdf]

# Appendix A to the paper #1538: Questions for respondents during focus groups interviews

Introduction about the research project, interviewers, goals of the research, and questions during the interview. Privacy and anonymity disclosure and approvals.

## 1. Introductory and warm-up questions:

- What is your AI focus in which domain? What is your previous experience with AI?
- Do you remember one interesting struggle that you (or your colleagues) had when working with data, AI/ML methods, benchmarking,...? Can you share any lessons that you learned during the solution / What helped or would help you during your struggles?

## 2. Work on solutions

- What do your AI experiments look like (What steps are they composed of)?
- If replication studies: When you replicate some study (base your research on existing work), what is the starting point and what is the process? Do you use any reproducibility or replicability tool or service (e.g., Papers with code/ Codeocean)? What would help you (can you think about a user story)?
- Which AI tools and methods do you use for your AI research and for which purposes: (You can look on this website for inspiration: <https://landscape.lfai.foundation/> ) Which AI tools and methods do you use for data management? Which AI tools and methods do you use for modeling? Which AI tools and methods do you use for programming? Which AI tools and methods do you use for prototyping? Which AI tools and methods do you use for benchmarking? Which AI tools and methods do you use for trusted and responsible AI? Which AI tools and methods do you use for user research? Which AI tools and methods do you use for pipelines/workflows? Which tools did you try and give up and why? (lack of time, resources, training etc)
- Which computational resources and infrastructure do you use for research? Are you satisfied with the infrastructure?

## 3. Searching for information and data

- How do you search for information resources to know the state of the art in the topic of your dissertation? How do you search for research information-papers, conferences? How do you search for education materials? How do you search for informal resources? How do you search for datasets? How do you search for source codes? How do you search for models? How do you search for benchmarks of models? How do you search for authorities? How do you search for existing solutions? Please, provide tips to existing tools and their improvements.
- What kind of metadata/tags (characteristics) would you need to better use or search in datasets? What kind of metadata would you need to better use or search in codes?

What kind of metadata would you need to better use or search in models? What kind of metadata would you need to better search in conferences and papers?

- How do you distinguish the high-quality AI resources?
- Where do you ask questions about research challenges that you cannot find answers to (beyond googling and outside of your community)? What do you miss in your professional community (consultant, other PhDs, at work...) and in the existing professional forums or social networks? Under which conditions and when would you engage in virtual professional conversations outside of your current community?

#### 4. Organization of resources

- How do you store and organize papers? How do you store and organize datasets? How do you store and organize codes and models for your experiments? Where do you write and organize notes about your experiments?
- Are those tools good enough/what is wrong with them? How would you like to organize them (can you think of a user story)?

#### 5. Publication and Dissemination

- Do you use any channels for dissemination of your research? How do you imagine a perfect solution to spread the word about your research, particularly to business people (can you think of a user story)?
- Do you also publish resources like codes, AI models, datasets or prototypes when you publish a research paper? Why/ If not, what prevents you from doing so? What kind of motivations would you need to do so?
